# Supplementary material for: Stepped Graphene-based Aharonov-Bohm Interferometers
Source: arXiv:1812.02845 source file (2019-06-20)
Supplement: Supplementary file 1 [file supplmaterials.pdf]

# Supplemental material for
# "Stepped Graphene-based Aharonov-Bohm Interferometers"

**V. Hung Nguyen and J.-C. Charlier**
*Institute of Condensed Matter and Nanosciences, Université catholique de Louvain,*
*Chemin des étoiles 8, B-1348 Louvain-la-Neuve, Belgium*

## Contents:

1. ***Computational methodologies***
2. ***Curvature-induced local strains in stepped graphene***
   *Local strains induced by curvature and simulated models are discussed.*
3. ***Tight Binding versus Density Functional Theory calculations***
   *Validity of tight binding model to investigate the local strains is considered by the fit to the density functional theory calculations*
4. ***Effects of curvature-induced local strains on Aharonov-Bohm interference***
5. ***Effects of edge disorder in graphene nanoribbons***
6. ***Multi sub-bands contribution***
   ***References***

---

## 1. Computational methodologies

In order to compute the electronic transport through stepped graphene systems, we employed the Green's function technique [1] to solve the tight-binding Hamiltonian presented in the main text. In particular, the retarded Green's function is determined as

$$G^R(E) = \left[E + i0^+ - H_D - \Sigma_L - \Sigma_R\right]^{-1} \quad \text{(S.1)}$$

where $H_D$ is the device Hamiltonian and $\Sigma_{L,R}$ are self-energies describing the left and right device-to-lead couplings, respectively. This equation was solved using the recursive method [2]. The transport quantities such as transmission probability $T(E)$, conductance $\mathcal{G}(E_F)$ and local density of left- and right-injected states $D_{L,R}(E,r)$ are then computed using the Landauer formalism as follows:

$$T(E) = Tr\left[\Gamma_L G^R \Gamma_R G^{R\dagger}\right] \quad \text{(S.2)}$$

$$\mathcal{G}(E_F) = \frac{2e^2}{h}\int_{-\infty}^{+\infty} dE\, T(E)\left(-\frac{\partial f_F}{\partial E}\right) \quad \text{(S.3)}$$

$$D_{L,R}(E,r) = \frac{G^R \Gamma_{L,R} G^{R\dagger}}{2\pi} \quad \text{(S.4)}$$

Here, $\Gamma_{L,R} = i\left[\Sigma_{L,R} - \Sigma^\dagger_{L,R}\right]$ and $f_F(E)$ is the Fermi-Dirac distribution function with the Fermi level $E_F$. The total local density of states can be computed either by $D(E,r) = D_L(E,r) + D_R(E,r)$ or $D(E,r) = -\Im(G^R)/\pi$.

## 2. Curvature-induced local strains in stepped graphene

In general, the non-planar geometry can induce in-plane strain inhomogeneities (i.e., local strains). Different from the uniform strains, local strains can result in electron scatterings and can be effectively described as the effects of strain-induced gauge fields in stepped graphene systems. These local strains have been shown to be often observed in the detached regions, i.e., around the step edges [3-5].

However, it has been experimentally demonstrated that if no external stress is applied, only small local strains can be observed in the stepped graphene systems, because of the mechanical robustness of graphene layers. For instance, it has been investigated and reported in refs. [3,4] that graphene at the step could experience small uniaxial strains (i.e., < 1%) relative to the rest of the sheet and **nearly strain-free graphene is possible in epitaxial graphene**. Extremely small strains of ~ 0.025% were also demonstrated in ref. [5] by Raman spectroscopy measurements.

To investigate the effects of such local strains induced by graphene curvature, we assume a simple model that the strain is maximum at the step edges and gradually release in two sides. Here, we use the following simple formula to model these strains:

$$\varepsilon(r)=\frac{\varepsilon_{max}}{1+(d/d_0)^2} \tag{S.5}$$

where $\varepsilon_{\max}$ is the maximum value of strain, $d$ is the in-plane distance from the position $\boldsymbol{r}$ to the considered step edge, and $d_0$ characterizes the strain release distance. Fig. S1 shows a typical picture of possible strain gradients induced by graphene curvature, that can be modelled by the above formula.

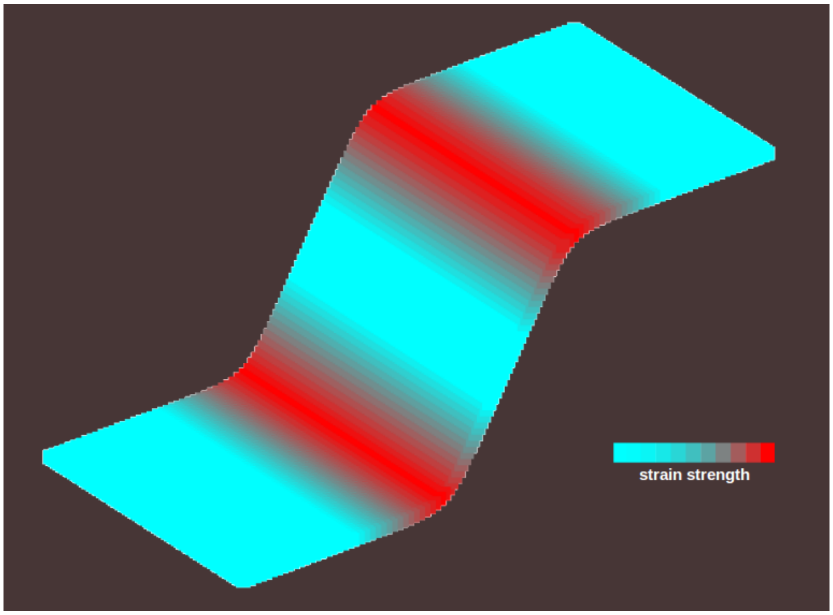


**Fig. S1**: *Possible local strains induced by curvature in stepped graphene systems.*

In next sections **3** and **4**, using such the simple model we present an investigation to clarify the effects of possible local strains mentioned above on the Aharonov-Bohm interference predicted in this work.

## 3. Tight Binding versus Density Functional Theory calculations

In this section, we present some calculations demonstrating the validity of the tight binding (TB) Hamiltonian to investigate the curvature-induced local strains in stepped graphene systems by the fit to the ab *initio* quantum transport data [6].

Actually, it has been shown by several studies in the literature that a simple $p_z$ TB Hamiltonian with only nearest neighbor interactions can be used to compute very accurately the electronic properties and electron transport in planar graphene systems. However, the curvature in the stepped graphene systems can alter their electronic properties, i.e., can induce electron scatterings, especially, when a local strain occur around the step edges as discussed above. Hence, the validity of the $p_z$ TB model is needed to be examined. To this aim, we performed quantum transport calculations based on density functional theory (DFT) [6] for stepped graphene systems, which are assumed very large so as to neglect the finite-width effects and hence the periodic boundary condition can be applied along Oy axis.

The transmission coefficients through stepped graphene systems obtained for three different $k_y$-momentum modes around the Dirac point are computed and presented in Fig. S2. Two cases without and with a local strain ($\varepsilon_{max}$ = 1%) are considered. In agreement with the study in [7] with different curvature radius, step heights and step angles, the results obtained without the local in-plane strain show that the effects of curvature on the electronic transport through the system is negligible. In particular, for $k_y = K_0$, the transmission coefficient exhibits only negligibly small reduction around the zero energy point, compared to the planar case where it is unity and constant in the considered energy range. Thus, the curvature does not induce significant electron scatterings and hence, similar to the planar cases, the $p_z$ TB Hamiltonian still works well for these considered stepped graphene systems.

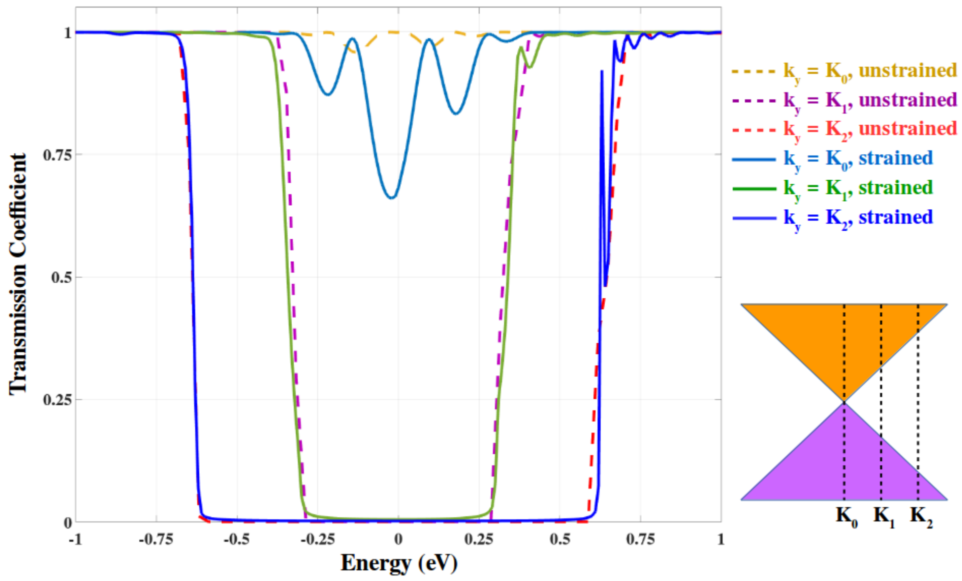


**Fig. S2**: *Electronic transport through stepped 2D graphene systems using DFT calculations: strained (with $\varepsilon_{max}$ = 1%) system as described in Fig.S1 versus unstrained one.*

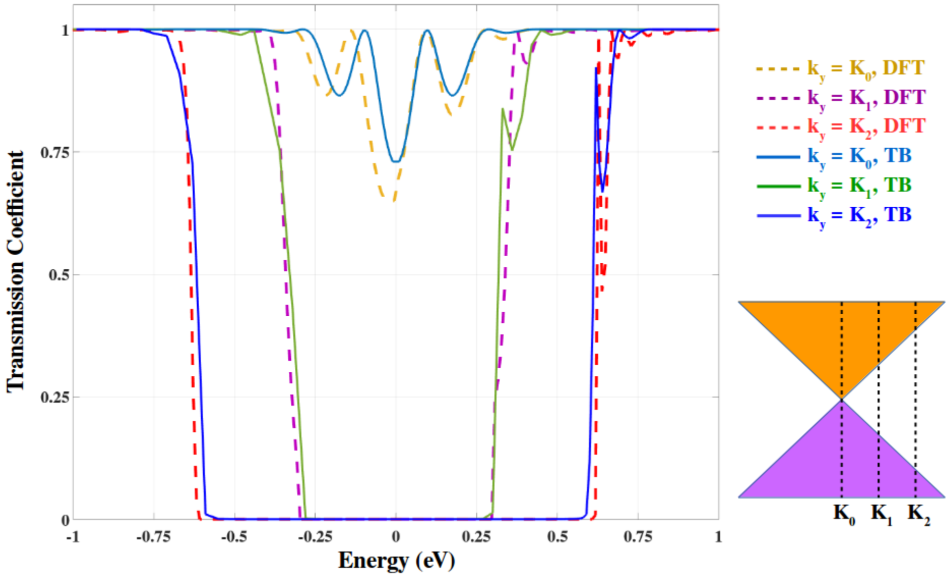


**Fig. S3**: *Electronic transport through stepped 2D graphene system with local strain $\varepsilon_{max}$ = 1%: Tight-Binding vs DFT calculations.*

When the curvature-induced local strains are introduced, significant electron scatterings at the step edges can be observed. Indeed, the transmission coefficient exhibits significant reduction around the zero energy point for $k_y = K_0$ mode and close to the edges of energy gap for other modes $K_{1,2}$. In order to compute these effects, the $p_z$ TB Hamiltonian must be adjusted. In particular, a model where the hopping term is determined a function of C-C bond length $r_{ij}$ as $t_{ij}=t_0\exp\left[\beta\left(1-r_{ij}/r_0\right)\right]$ with $\beta$=3.37 and $r_0$ = 0.142 nm has been demonstrated [8] to compute well the strain effects in graphene. Fig. S3 demonstrates a quite good agreement between the DFT data and results obtained by such strained TB model. Our calculations show that this strained TB Hamiltonian without any other adjustment is still a good model for the considered stepped graphene systems with local strains of $\varepsilon_{max} \lesssim 4\%$.

## 4. Effects of curvature-induced local strains on Aharonov-Bohm interference

In this section, we employed the strained TB model presented above to investigate the effects of curvature-induced local strains in the Aharonov-Bohm interferometers predicted in this work.

The conductance as a function of Fermi energy obtained at zero magnetic field is presented in Fig. S4. Similar to the results presented in section **3**, the considered local strain can induce electron scatterings and affect significantly the transport through the system, leading to the conductance reduction.

The effects of such strains on the predicted Aharonov-Bohm interference are investigated and presented in Fig. S5. It is however shown that the effects on the conductance oscillations in the quantum Hall regime are relatively weaker than those observed in the low field one. This can be explained as follows. In the low field regime, the electron transport is essentially due to “bulk states”, which transmit across the step edges (i.e., zones of local strains) and hence undergo strong back-scatterings as described in the top-right image of Fig.S5. In the quantum Hall regime, the presence of these locally strained zones however affects the transport picture differently. In particular, when a high magnetic field with $\theta_B < \theta_S$ is applied, opposite edge states are formed in terrace and facet zones (in two sides of the step edges) and electrons transmitting through the system have to follow trajectories as described in the bottom-

right image of Fig.S5, i.e., when reaching the step edges, electrons transmit along (not directly across, as in the zero-field case) these edges. This can eliminate the scatterings induced by the considered local strains and explain their weak effects in the quantum Hall regime, compared to those in the low field one. Hence, within the range of experimentally reported strains discussed above, the considered local strains even though alter but does not strongly perturb the predicted Aharonov-Bohm interference.

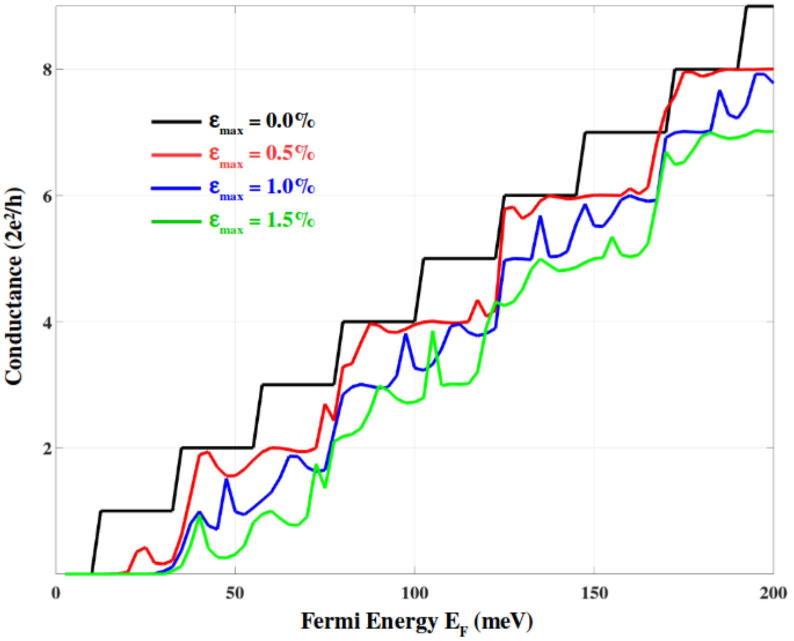


**Fig. S4**: *Conductance as a function of energy at zero magnetic field with different curvature-induced strains. The strain release distance $d_0 \approx 11$ nm while other parameters are as in Fig.2 of the main text.*

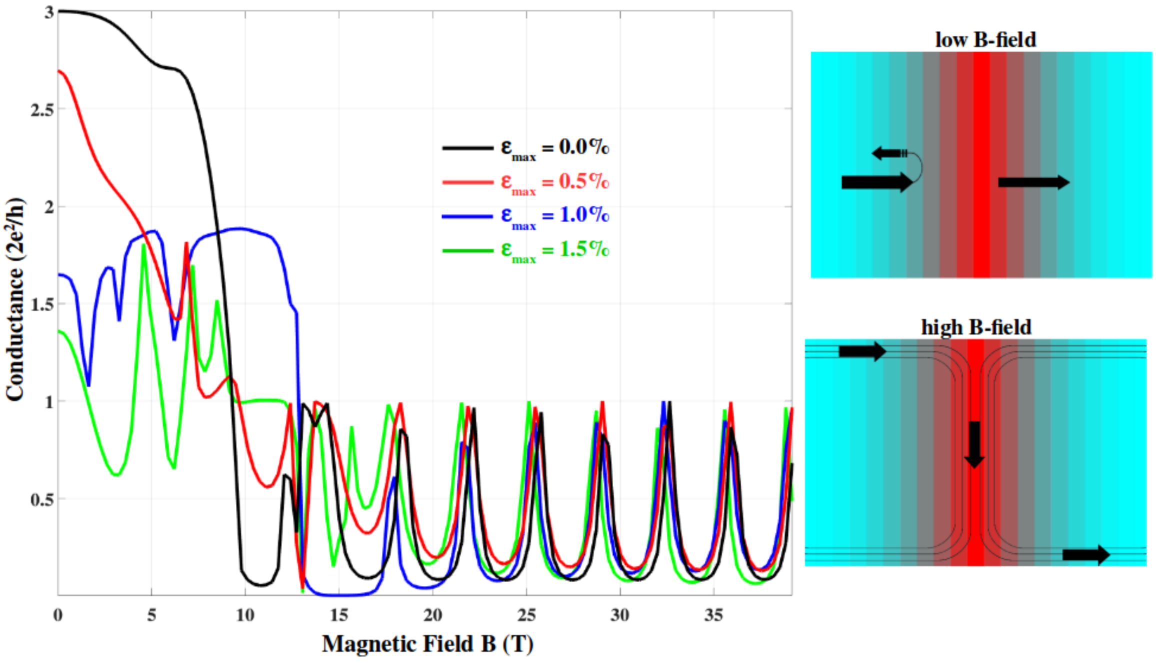


**Fig. S5**: *Conductance as a function of magnetic field at $E_F$ = 75 meV and with different curvature-induced strains. Parameters are as in Fig.S4. Right panels illustrate the electron transport pictures at low and high magnetic fields.*

Certainly, the effects of these local strains on the Aharonov-Bohm interference can be enlarged and significant when much larger strain gradients occur, for instance, when external stresses are additionally applied.

## 5. Effects of edge disorder in graphene nanoribbons

Similar to the surface roughness in many nanoscale systems of conventional semiconductors, the edge disorder (i.e., edge roughness) is often a practical issue for graphene ribbons [9-19]. The edge disorder has been shown to affect strongly the electronic transport through graphene ribbons, especially, when their width reaches the nanoscale regime.

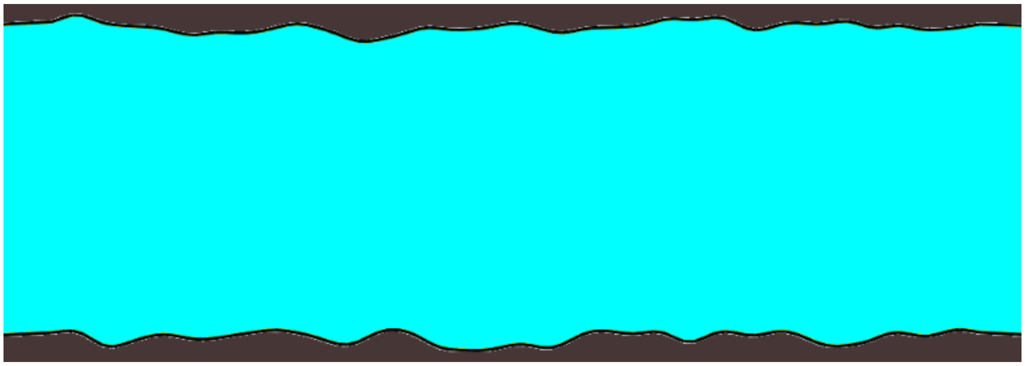

**Fig. S6**: *Graphene ribbon with edge disorder.*

To investigate the effects of edge disorder, there were two models widely used in the literature. In particular, the disordered edges can either be generated by randomly removing the edge atoms with a certain probability [11-14] or are modeled using auto-correlation functions [15-19]. These models have been demonstrated to interpret well the electronic properties of GNRs in experiments with a wide range of disorder level [9-19]. Here, the effects of edge disorder are examined using both two models. In the latter case, the edge disorder is generated by a Gaussian autocorrelation function, particularly, the variation of ribbon width $\delta W$ is effectively described as

$$\langle \delta W(x)\,\delta W(x+\Delta x)\rangle = W_{rms}^2 \exp\left(-\frac{\Delta x^2}{2\xi^2}\right) \qquad \text{(S.6)}$$

where $W_{rms}$ is the rms value charactering the disorder strength and $\xi$ represents the correlation length.

A typical picture of edge disordered graphene ribbons is illustrated in Fig. S6. The effects of edge disorder generated by a Gaussian autocorrelation function are presented in Fig. 4 of the main text and the results obtained in the systems by randomly removing edge atoms are displayed in Fig. S7.

**Actually, two main features are found with both disorder models.**

First, in the case of semiconducting GNRs, the Aharonov-Bohm oscillations obtained at high magnetic fields (*B*-fields) are shown to be much more robust under the effect of the considered disorders than the zero-field transport. This can be explained by a fascinating feature that different from the zero-field case (see Figs.S8 (a,d)), the forward and backward edge channels are spatially separated in the quantum Hall regime (see Figs.S8 (b-c, e-f)) while the scatterings at the disordered edges do not allow electrons

to transmit across the sample. As a consequence, the edge disorder effects do not contribute significantly to backscatterings in the considered stepped systems, i.e., the dominant mechanism of backscattering is still interaction between edge states in zones of opposite normal *B*-fields and hence strong Aharonov-Bohm oscillations are still achieved.

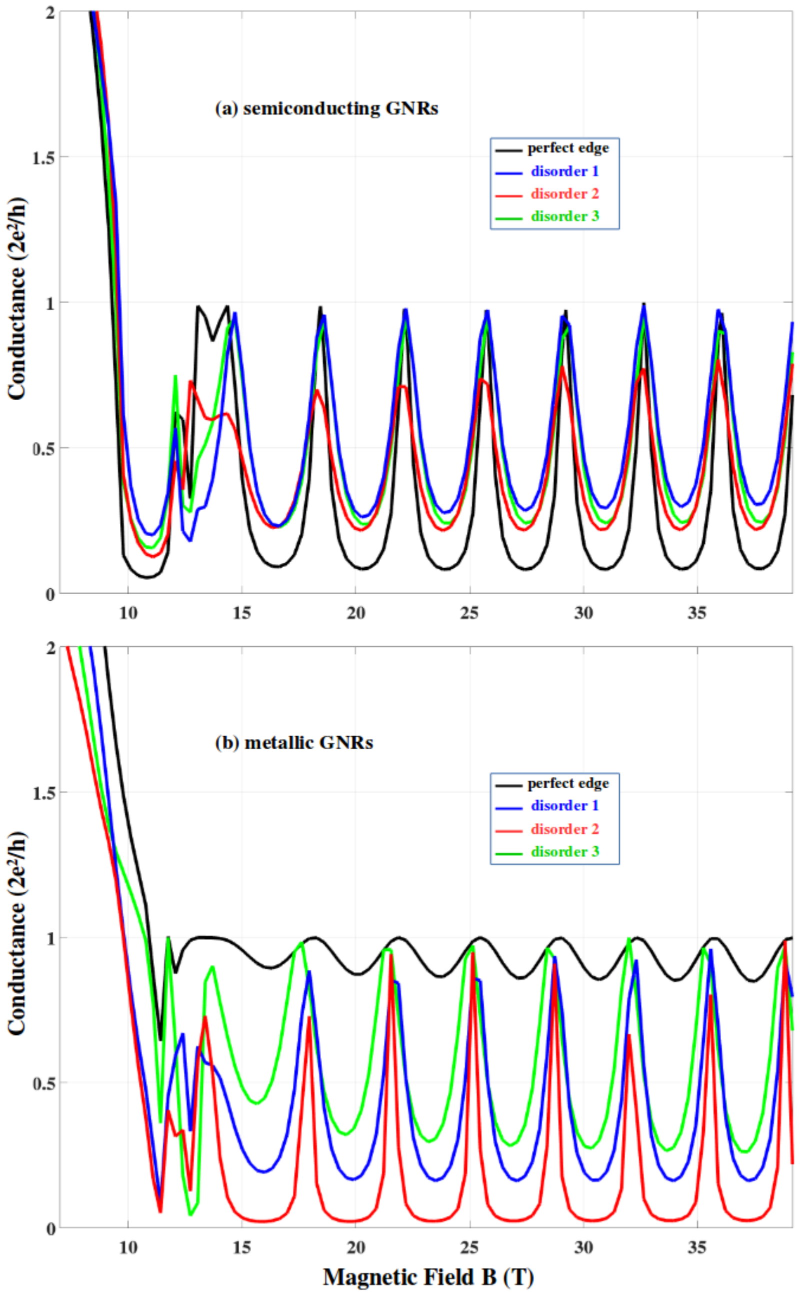


**Fig. S7**: *(a,b) Conductance as a function of B-field at* $E_F$ *= 75 meV computed for semiconducting (*$N_z$ *= 324) and metallic (*$N_z$ *= 326) GNR systems, respectively, with* $\theta_S = 60°$, $\theta_B = 30°$, $L_F \approx 75$ *nm and* $W \approx 40$*nm. In the edge disordered systems, 15% of edge atoms are randomly removed.*

Second, as presented in Fig.4 of the main text and in Fig. S7, there is a significant difference between semiconducting and metallic GNR systems with perfect edges, i.e., the Aharonov-Bohm oscillation is relatively weak in the metallic cases, compared to the results obtained in semiconducting ones. The

edge disorder however strengthens the Aharonov-Bohm oscillation in metallic GNR systems, thus eliminating the difference mentioned.

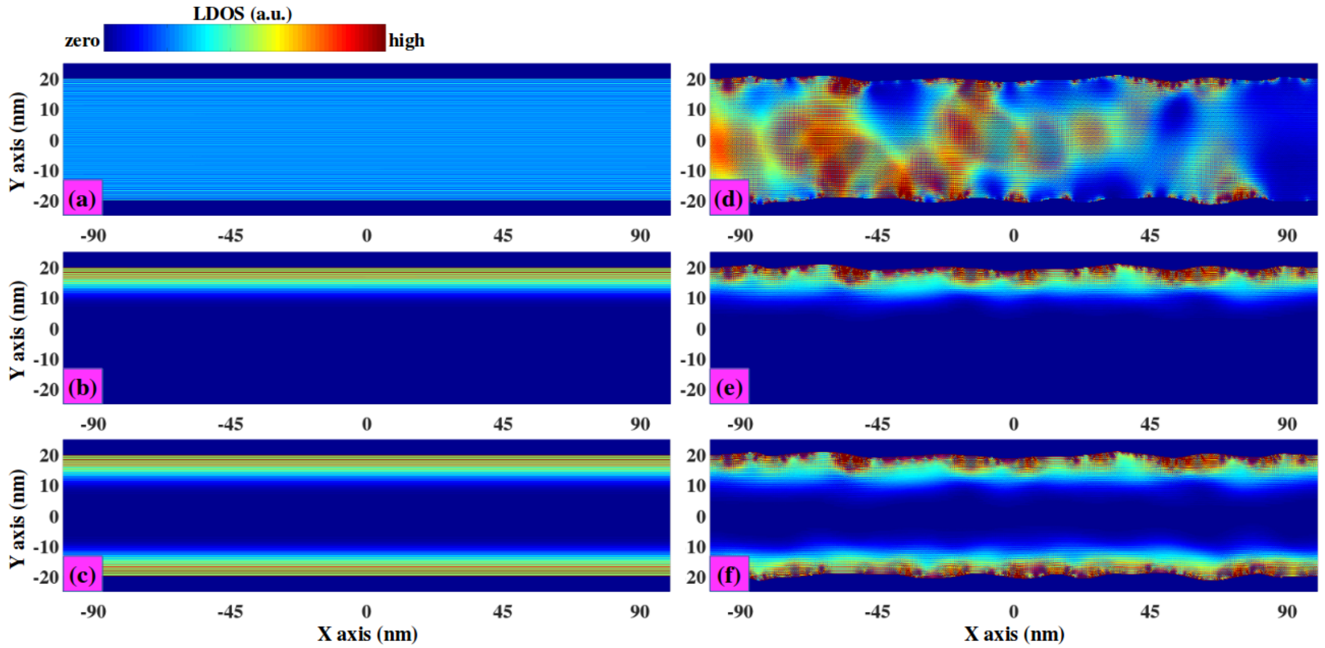


**Fig. S8**: *Edge disorder effects on electron propagation in planar graphene ribbons: left-injected LDOS (a,b,d,e) and total LDOS (c,f). Magnetic fields B = 0 in (a,d) and 25 T in (b,c,e,f) while carrier energy E = 75 meV. Perfect and disordered edges are considered in (a,b,c) and (d,e,f), respectively.*

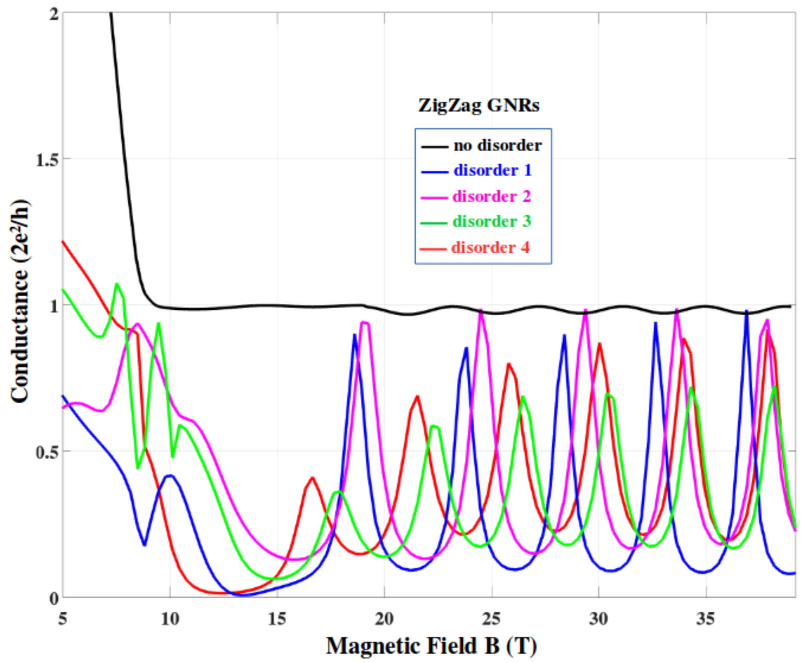


**Fig. S9**: *Conductance as a function of B-field at $E_F$ = 75 meV obtained in stepped systems of a zigzag GNR with $\theta_S$ = 60°, $\theta_B$ =30°, $L_F \approx$ 72 nm and W ≈ 40 nm. The disordered edge systems are generated by the Gaussian autocorrelation function (S.6) with $W_{rms} \approx$ 0.6 nm and $\xi \approx$ 4.8 nm.*

Note additionally that a picture, similar to those obtained in the metallic armchair GNRs, is also observed in zigzag GNR systems, i.e., the Aharonov-Bohm oscillation is relatively weak for perfect edges but the effect is much more pronounced when edge disorder is introduced (see Fig. S9).

## 6. Multi sub-bands contribution

In this section, we analyze the effects of multi sub-bands contribution on the predicted Aharonov-Bohm oscillation in more detail. As it has been demonstrated in nanorings [20,21] and also in graphene *p-n* junctions [22], the Aharonov-Bohm interference has an inherent property that the strong oscillation of conductance can be observed in the low energy regime where only a single band is obtained. In the regime of high energies when multi energy bands can contribute to the transport, the interference picture can be significantly blurred. A similar feature is also observed in the Aharonov-Bohm interferometers considered here.

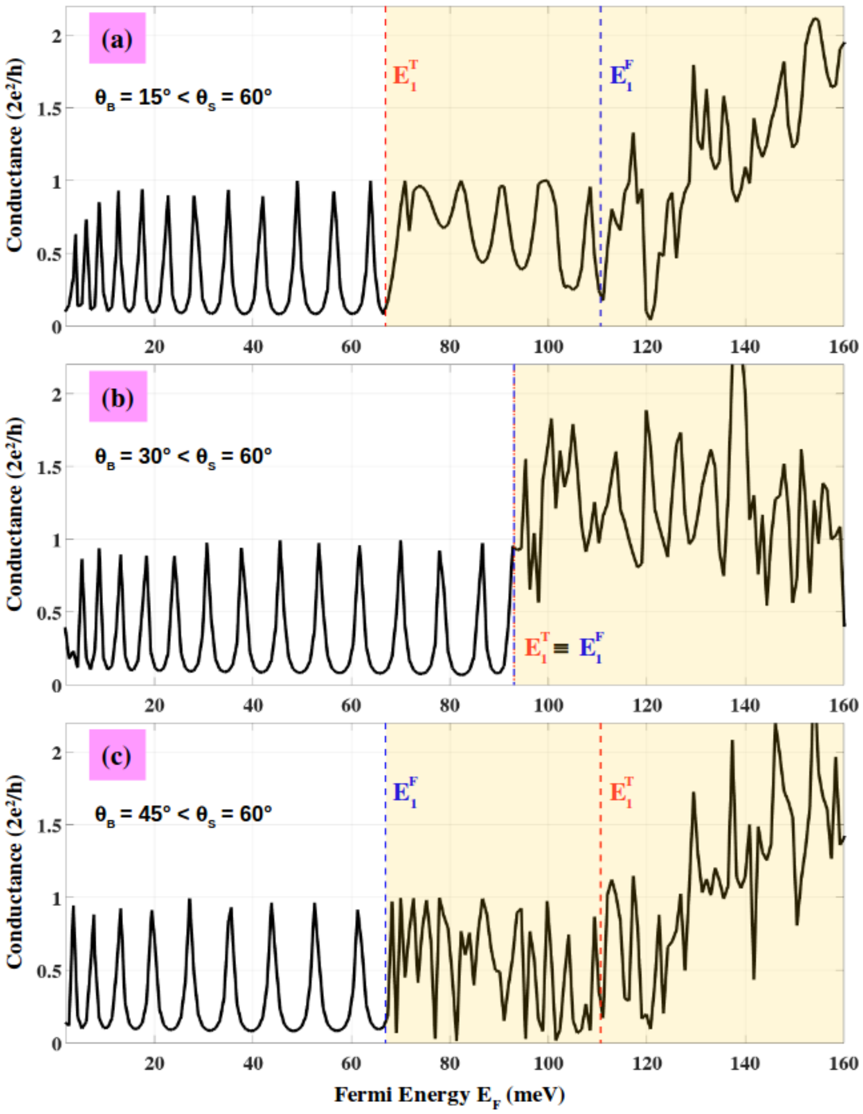


**Fig. S10**: *Conductance as a function of Fermi energy at B = 20 T obtained in stepped systems of an armchair GNR with $L_F \approx 110$ nm and $W \approx 60$ nm. The stepped angle $\theta_S = 60°$ while three directions of B-field are considered. $E_1^{T(F)}$ indicates the first Landau level formed in the terrace (facet) zone.*

Indeed, as shown in Fig. S10 and Fig. 5 of the main text, strong conductance oscillations in all considered cases are observed in the regime $E_F \le min(E_1^T, E_1^F)$ where $E_1^{T,F}$ are the first Landau levels formed in the terrace and facet zones, respectively, at high magnetic fields. In Fig. S11, the energy bands of an armchair GNR under the effect of magnetic field are presented. When a high magnetic field is applied, the energy bands of GNR are strongly modified and the Landau quantization is observed as seen in the right panel of Fig.S11. This Landau quantization (i.e., energy levels $E_{0,\pm1,\pm2,...}$) obeys the well-known formula [23]

$$E_n = sign(n)\sqrt{2e\hbar v_F^2 |n| B_\perp} \tag{S.7}$$

where $v_F$ is the Fermi velocity in graphene. The energy levels $E_1^T$ and $E_1^F$ mentioned above are hence determined as $E_1^T = \sqrt{2e\hbar v_F^2 B|\sin\theta_B|}$ and $E_1^F = \sqrt{2e\hbar v_F^2 B|\sin(\theta_S - \theta_B)|}$.

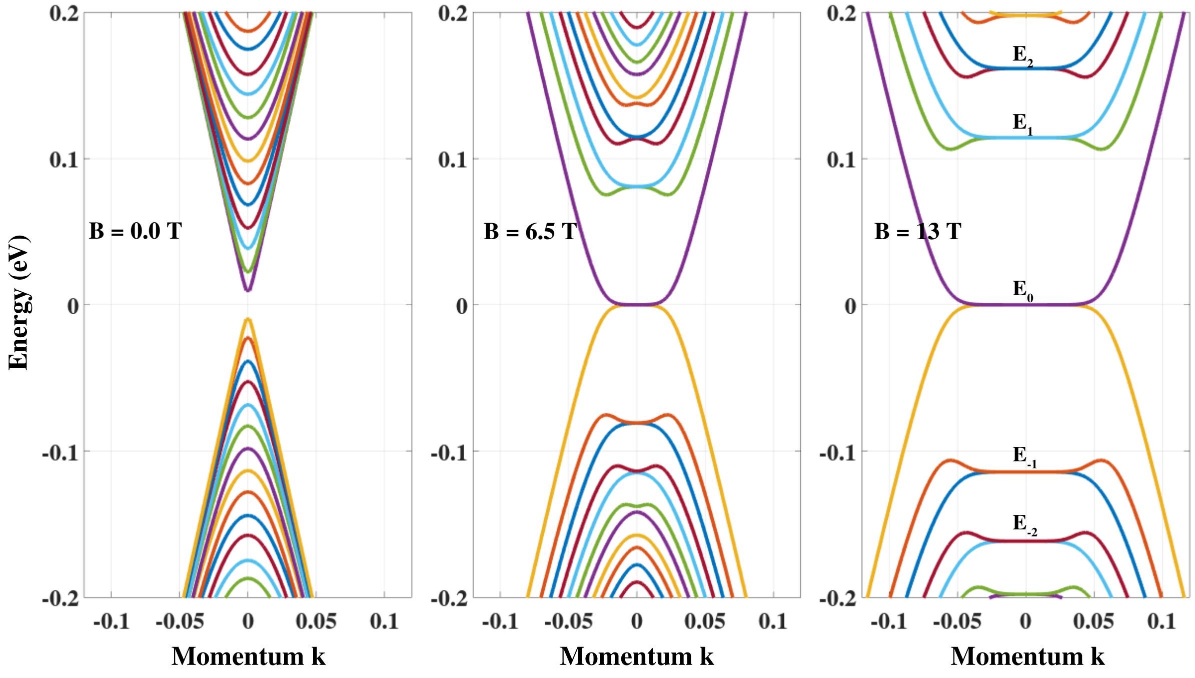


**Fig. S11**: *Energy bands of the armchair GNR of W ≈ 60 nm under the effect of magnetic field. Energy levels $E_n$ (n=0,±1,±2,...) in the right panel represent the Landau quantization at a high B-field [23].*

In the high energy regime, the effects of multi sub-bands contribution, similar to those observed in graphene and phosphorene nanorings [20,21] and mentioned above, are clearly demonstrated in Fig.S10 (see the zones highlighted in yellow). In general, the Aharonov-Bohm oscillations are significantly blurred by such contribution when $E_F > min(E_1^T, E_1^F)$, as illustrated in both Fig. S10 here and Fig.5 of the main text. In the cases if $E_1^T \neq E_1^F$ (e.g., $\theta_B$ = 15° and 45°), some oscillations can still be well defined in the range between these two values (see Fig. S10 for $\theta_B$ = 15°).

The features presented here explain clearly the results presented and discussed in Fig.5 of the main text.

## References:


[1] V. Hung Nguyen *et al.*, J. Comput. Electron. **12**, 85-93 (2013).
[2] C. H. Lewenkopf and E. R. Mucciolo, J. Comput. Electron. **12**, 203-231 (2013).
[3] J. A. Robinson *et al.*, Nano Lett. **9**, 964-968 (2009).
[4] T. Low, V. Perebeinos, J. Tersoff, and Ph. Avouris, Phys. Rev. Lett. **108**, 096601 (2012).
[5] B. D. Briggs *et al.*, Appl. Phys. Lett. **97**, 223102 (2010).
[6] http://www.openmx-square.org
[7] Y. Xu, H. Gao, M. Li, Z. Guo, H. Chen, Z. Jin and B. Yu, Nanotechnol. **22**, 365202 (2011).
[8] V. M. Pereira, A. H. Castro Neto, and N. M. R. Peres, Phys. Rev. B **80**, 045401 (2009).
[9] M. Y. Han, B. Özyilmaz, Y. Zhang, and P. Kim, Phys. Rev. Lett. **98**, 206805 (2007).
[10] M. Y. Han, J. C. Brant, and P. Kim, Phys. Rev. Lett. **104**, 056801 (2010).
[11] M. Evaldsson *et al.*, Phys. Rev. B **78**, 161407(R) (2008).
[12] D. Querlioz *et al.*, Appl. Phys. Lett. **92**, 042108 (2008).
[13] A. Cresti and S. Roche, New J. Phys. **11**, 095004 (2009).
[14] M. Poljak and T. Suligoj, IEEE Trans. Electron Devices **63**, 537-543 (2016).
[15] M. V. Fischetti and S. Narayanan, J. Appl. Phys. **110**, 083713 (2011).
[16] N. Djavid *et al.*, IEEE Trans. Electron Devices **61**, 23 - 29 (2014).
[17] T. Misawa *et al.*, Jpn. J. Appl. Phys. **54**, 05EB01 (2015).
[18] T. Fang, A. Konar, H. Xing, and D. Jena, Phys. Rev. B **78**, 205403 (2008).
[19] A. Y. Goharrizi *et al.*, IEEE Trans. Electron Devices **58**, 3725 - 3735 (2011).
[20] V. Hung Nguyen, Y. M. Niquet, and P. Dollfus, Phys. Rev. B **88**, 035408 (2013).
[21] R. Zhang, Z. Wu, X. J. Li, and K. Chang, Phys. Rev. B **95**, 125418 (2017).
[22] A. Mreńca-Kolasińska, S. Heun, and B. Szafran, Phys. Rev. B **93**, 125411 (2016).
[23] L.-J. Yin, K.-K. Bai, W.-X. Wang, S.-Y. Li, Y. Zhang, and L. He, Front. Phys. **12**, 127208 (2017).
